# Supplementary material for: Efficient and Robust Estimation of Linear Regression with Normal Errors
Source: arXiv:1909.07719 source file (2019-09-17)
Supplement: Supplementary file 1 [file Supplemental_Material_AppABC_Efficient_and_Robust_Linear_Regression.pdf]

# Supplemental Material
# Appendices A, B and C for:
# Efficient and Robust Estimation of Linear Regression with Normal Errors

Alain Desgagné
Département de mathématiques, Université du Québec à Montréal, Montréal, Canada, desgagne.alain@uqam.ca

September 16, 2019

## A Proof that the FLP is well defined as a probability distribution (Section 2 of the main article)

**Proposition 1.** *The density $f_{\mathcal{FLP}}(y \mid \omega, \mu, \sigma)$ integrates to 1.*

*Proof.* Without loss of generality, we set $\mu = 0$, $\sigma = 1$ and $y = z$. We have

$$\begin{aligned}\int_{-\infty}^{\infty} f_{\mathcal{FLP}}(z \mid \omega, \mu, \sigma) dz &= (1-\omega)^{-1} \left[ 2\omega\varphi(\tau)\tau \int_{\tau}^{\infty} \frac{1}{z} \left( \frac{\log \tau}{\log z} \right)^{\lambda+1} dz - 2\omega \int_{\tau}^{\infty} \varphi(z) dz \right] \\ &= (1-\omega)^{-1} \left[ 2\omega\varphi(\tau)\tau(\log\tau)\lambda^{-1} - \omega(1-\rho) \right] = 1 \\ &\Leftrightarrow 2\omega\varphi(\tau)\tau(\log\tau)\lambda^{-1} = 1 - \omega\rho \Leftrightarrow \lambda = 2(1-\omega\rho)^{-1}\omega\varphi(\tau)\tau\log\tau,\end{aligned}$$

using the equation of $\rho$ in the second equality. □

**Proposition 2.** *A sufficient condition to obtain $f_{\mathcal{FLP}}(y \mid \omega, \mu, \sigma) > 0$ for $|z| > \tau$ and $0 < \omega < 1$ is given by $\tau > 1$, $(\tau^2 - 1)\log\tau > 1$ (or equivalently $\tau > 1.69901$) and $\omega \leq g(\tau)$.*

*Proof.* Without loss of generality, we set $\mu = 0$, $\sigma = 1$ and $y = z$. The condition $\tau > 1$ ensures that $\log z > 0$ for all $z \geq \tau$. By symmetry of the density, we just need to show that, for $z > \tau$,

$$f_{\mathcal{FLP}}(z \mid \omega, \mu, \sigma) > 0 \Leftrightarrow \frac{\varphi(\tau)}{\varphi(z)} \frac{\tau}{z} \left( \frac{\log\tau}{\log z} \right)^{\lambda+1} > 1 \Leftrightarrow h(z) > h(\tau),$$

where

$$h(z) := z^2/2 - \log z - (\lambda+1)\log\log z.$$

We observe that $h(z)$ is convex for all $z > \tau$ since

$$\frac{d^2}{dz^2} h(z) = 1 + z^{-2} + (\lambda+1)(\log z + 1)(z\log z)^{-2} > 0 \text{ for all } z > 1.$$

Thus

$$
\begin{aligned}
h(z) > h(\tau) \text{ for } z > \tau \Leftrightarrow \frac{d}{dz}h(z)\Big|_{z=\tau} \geq 0 &\Leftrightarrow \tau - \tau^{-1} - (\lambda+1)(\tau\log\tau)^{-1} \geq 0 \\
&\Leftrightarrow \lambda \leq (\tau^2-1)\log\tau - 1 \\
&\Leftrightarrow 2(1-\omega\rho)^{-1}\omega\varphi(\tau)\tau\log\tau \leq (\tau^2-1)\log\tau - 1 \\
&\Leftrightarrow \omega \leq \left(\rho + \frac{2\varphi(\tau)\tau\log\tau}{(\tau^2-1)\log\tau - 1}\right)^{-1} = g(\tau).
\end{aligned}
$$

Note that the condition $(\tau^2-1)\log\tau-1 > 0$ ensures that the inequality $\lambda \leq (\tau^2-1)\log\tau-1$ is not in contradiction with $\lambda > 0$. □

The contaminating distribution $\mathcal{FLP}(\omega, \mu, \sigma)$ is thus well defined as a probability distribution. We see in Proposition 1 that the equation of $\lambda$ ensures that its density integrates to 1 and we see in Proposition 2 that it suffices to set $\omega = g(\tau) \Leftrightarrow \tau = g^{-1}(\omega)$ to obtain a positive density.

# B Proof of the equivalence of the distances (Section 5 of the main article)

We have

$$
\begin{aligned}
(\hat{\boldsymbol\beta}-\boldsymbol\beta)^T(\mathbf{x}^T\mathbf{x})(\hat{\boldsymbol\beta}-\boldsymbol\beta) &= (\hat{\boldsymbol\beta}-\boldsymbol\beta)^T(\mathbf{x}_1,\ldots,\mathbf{x}_n)(\mathbf{x}_1,\ldots,\mathbf{x}_n)^T(\hat{\boldsymbol\beta}-\boldsymbol\beta) \\
&= (\hat{\boldsymbol\beta}-\boldsymbol\beta)^T(\mathbf{x}_1\mathbf{x}_1^T+\ldots+\mathbf{x}_n\mathbf{x}_n^T)(\hat{\boldsymbol\beta}-\boldsymbol\beta) = \sum_{i=1}^n(\hat{\boldsymbol\beta}-\boldsymbol\beta)^T\mathbf{x}_i\mathbf{x}_i^T(\hat{\boldsymbol\beta}-\boldsymbol\beta) \\
&= \sum_{i=1}^n\left(\mathbf{x}_i^T(\hat{\boldsymbol\beta}-\boldsymbol\beta)\right)^2 = \sum_{i=1}^n\left(\mathbf{x}_i^T\hat{\boldsymbol\beta}-\mathbf{x}_i^T\boldsymbol\beta\right)^2 = \sum_{i=1}^n(\hat\mu_i-\mu_i)^2.
\end{aligned}
$$

# C Monte Carlo simulations

The 22 graphs in the Monte Carlo simulations from Section 5 of the main article are presented below.

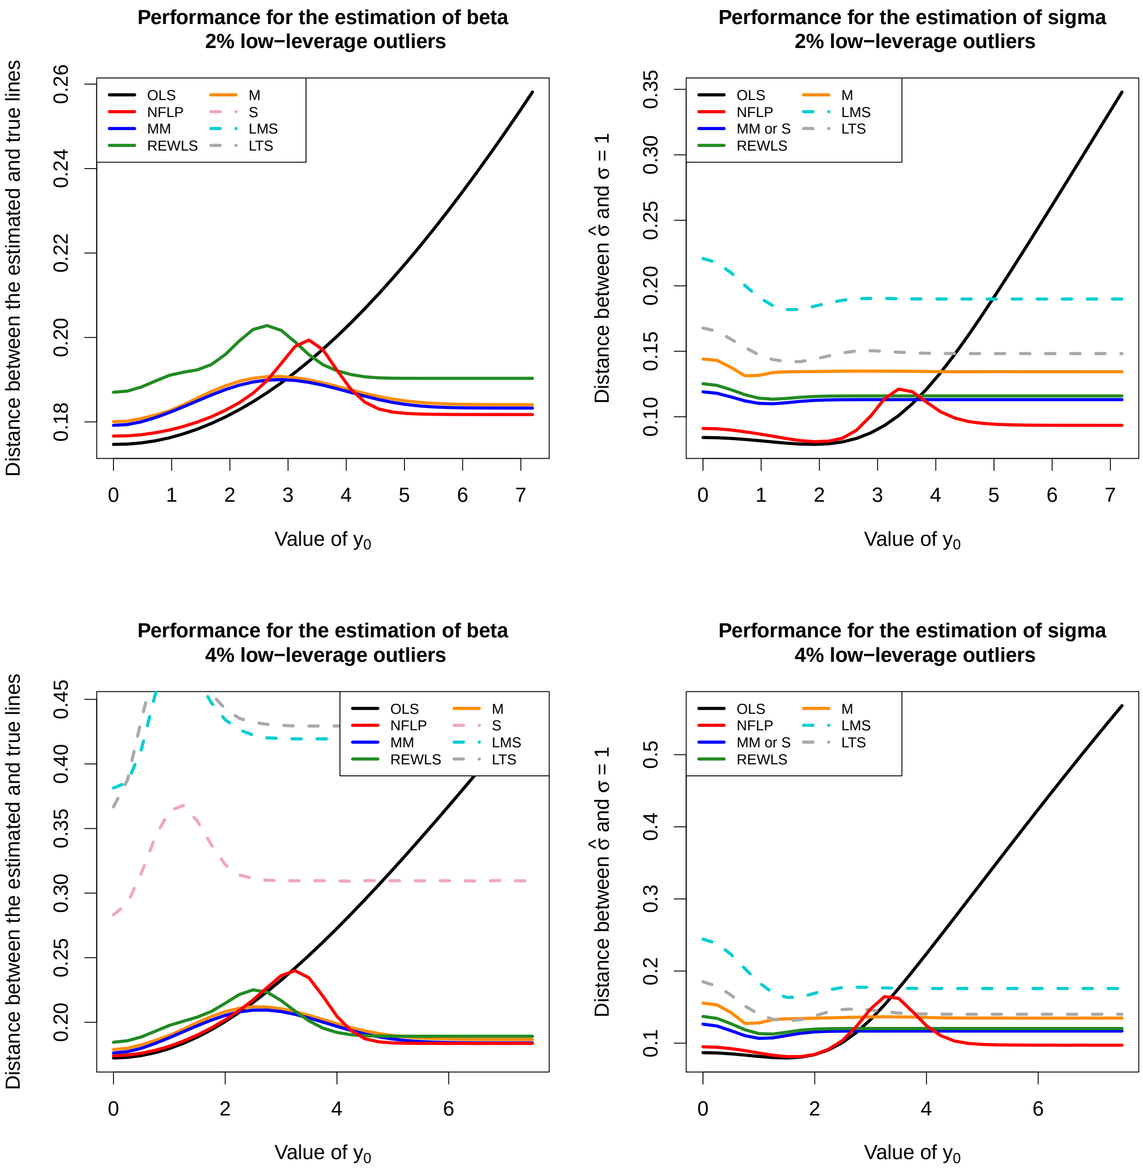


Figure 1: Performance of the estimators of $\boldsymbol{\beta}$ (left) and $\sigma$ (right) against 2% (top) and 4% (bottom) low-leverage outliers

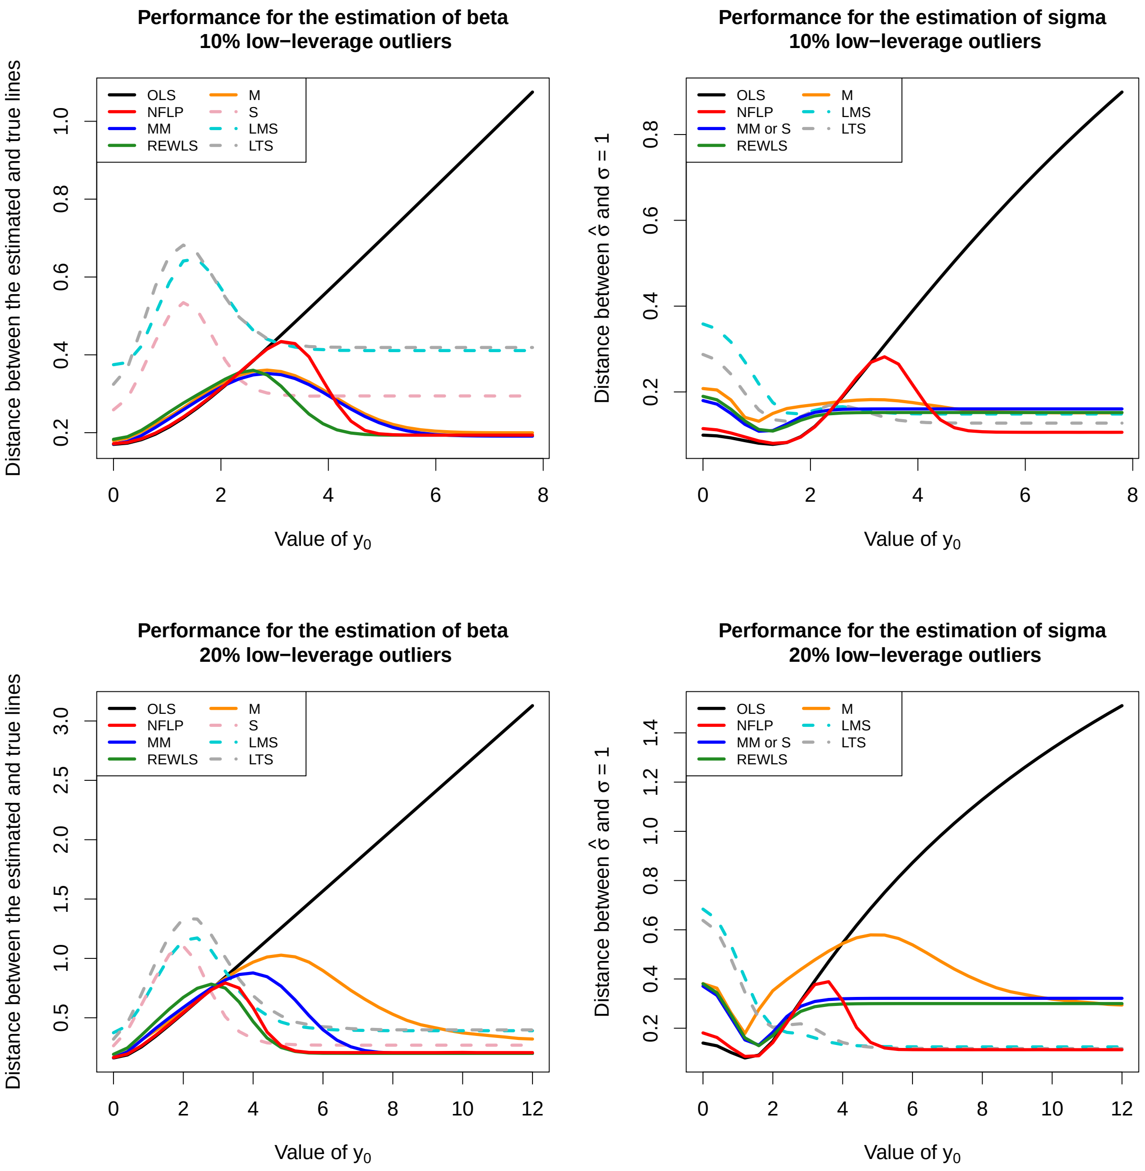


Figure 2: Performance of the estimators of $\boldsymbol{\beta}$ (left) and $\sigma$ (right) against 10% (top) and 20% (bottom) low-leverage outliers

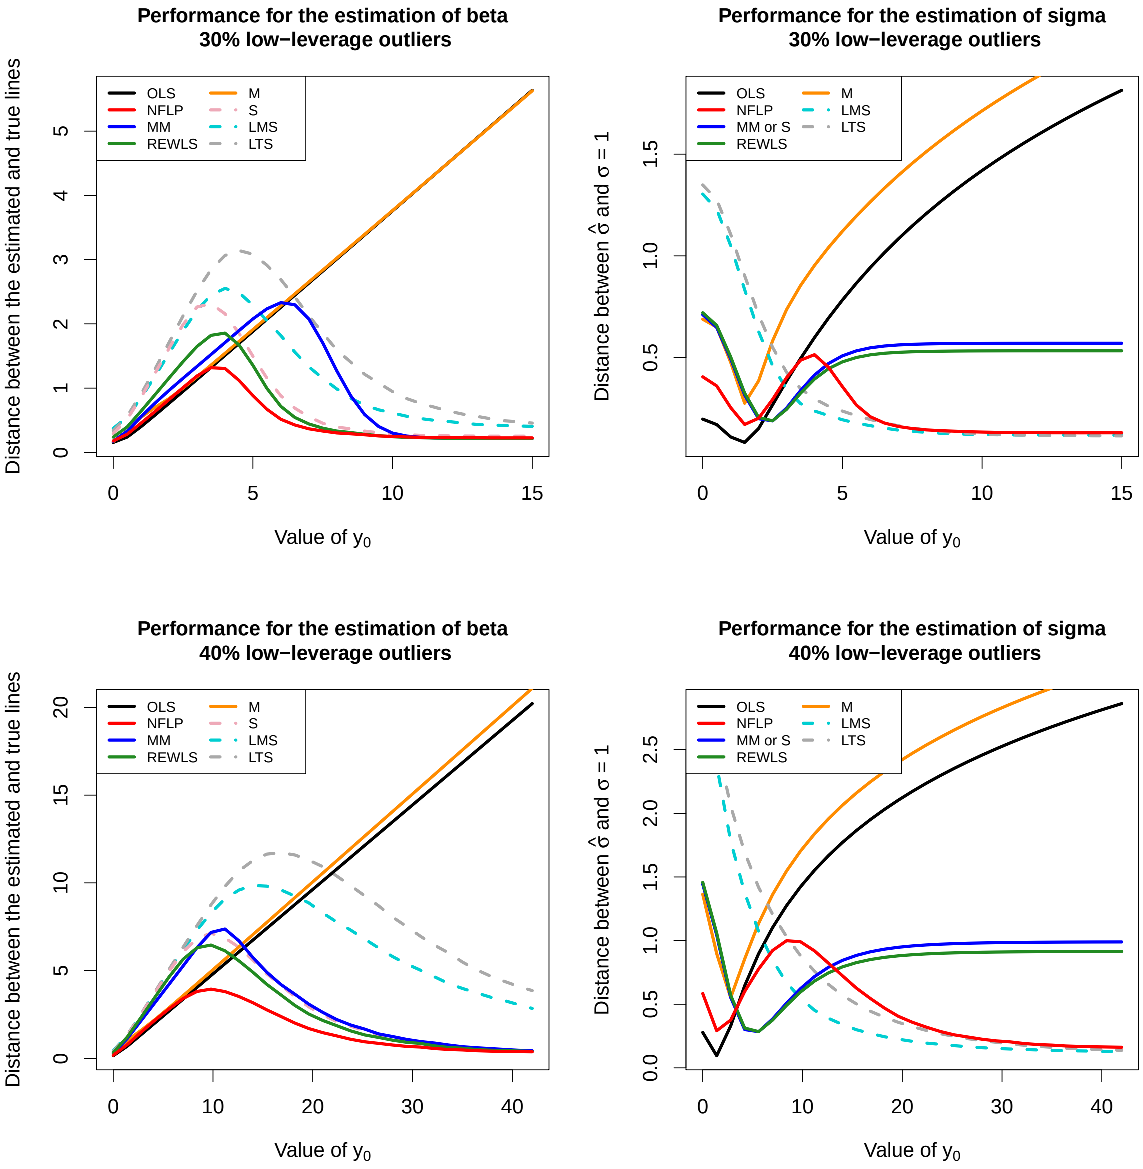


Figure 3: Performance of the estimators of $\boldsymbol{\beta}$ (left) and $\sigma$ (right) against 30% (top) and 40% (bottom) low-leverage outliers

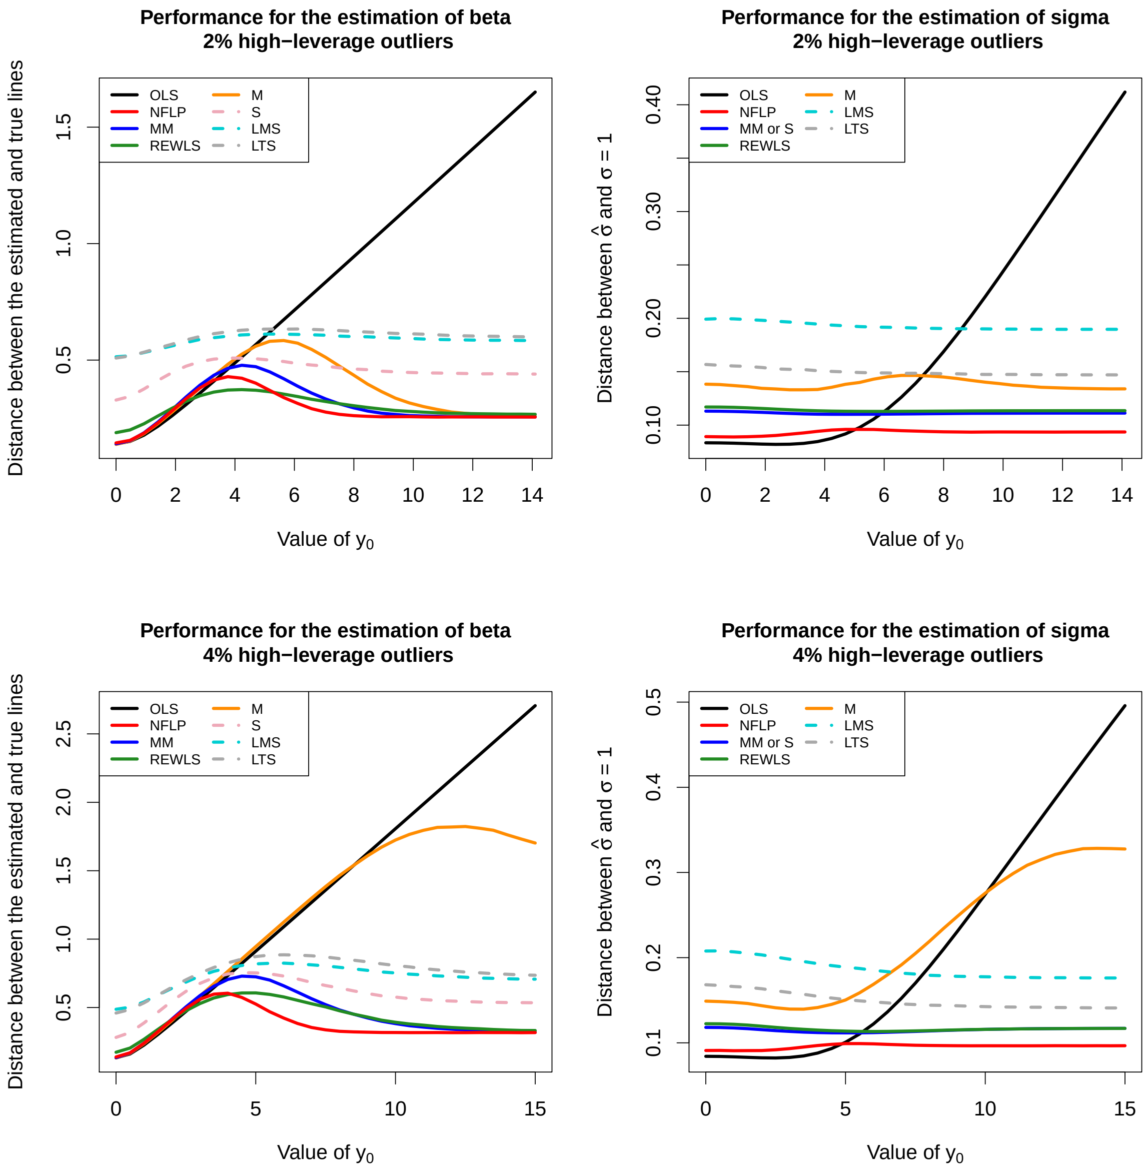


Figure 4: Performance of the estimators of $\boldsymbol{\beta}$ (left) and $\sigma$ (right) against 2% (top) and 4% (bottom) high-leverage outliers

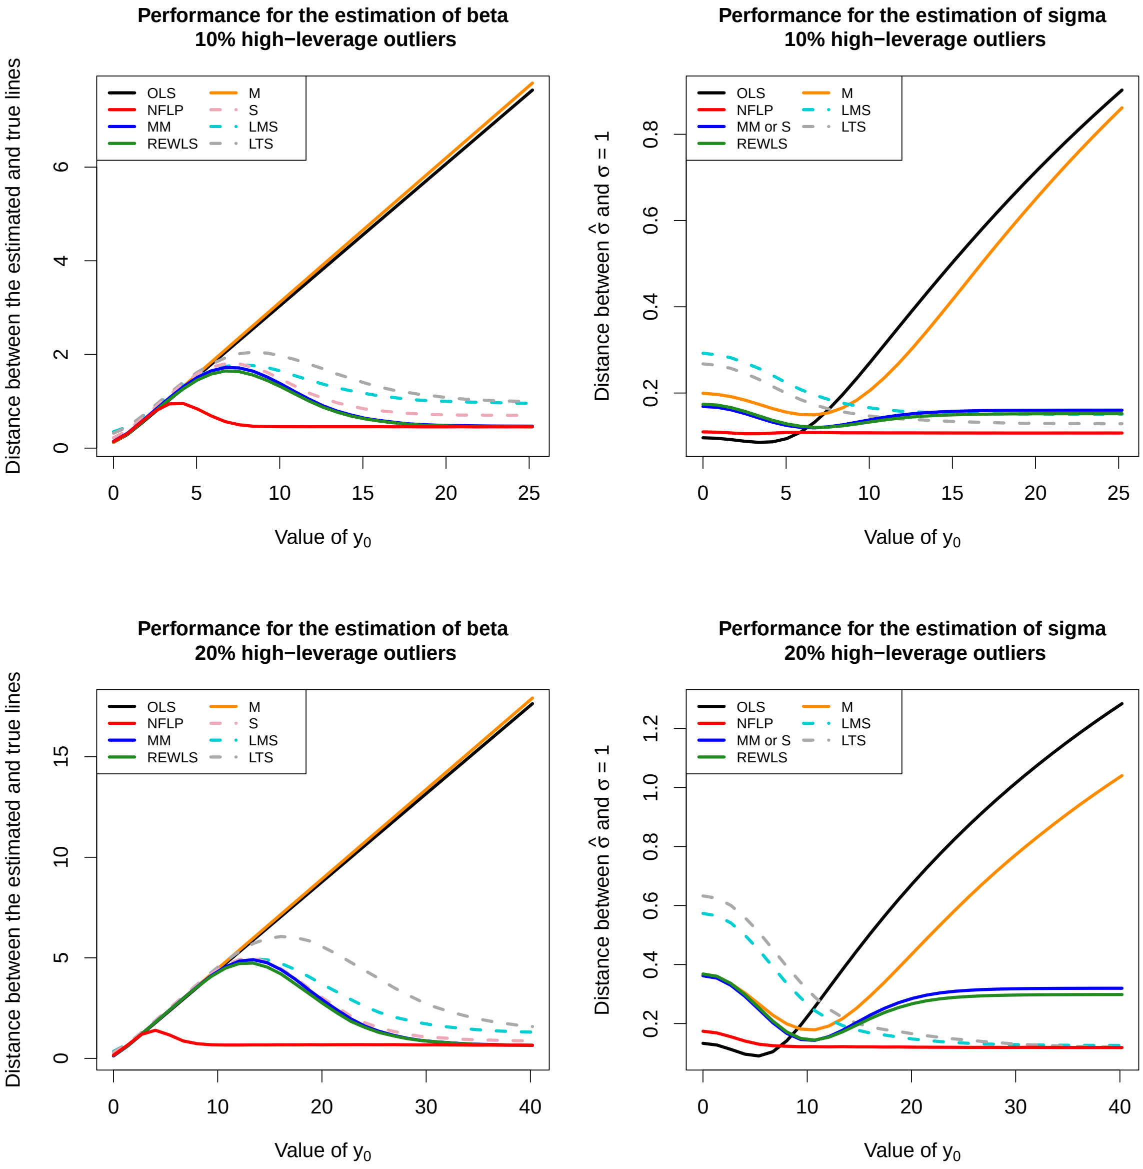


Figure 5: Performance of the estimators of $\boldsymbol{\beta}$ (left) and $\sigma$ (right) against 10% (top) and 20% (bottom) high-leverage outliers

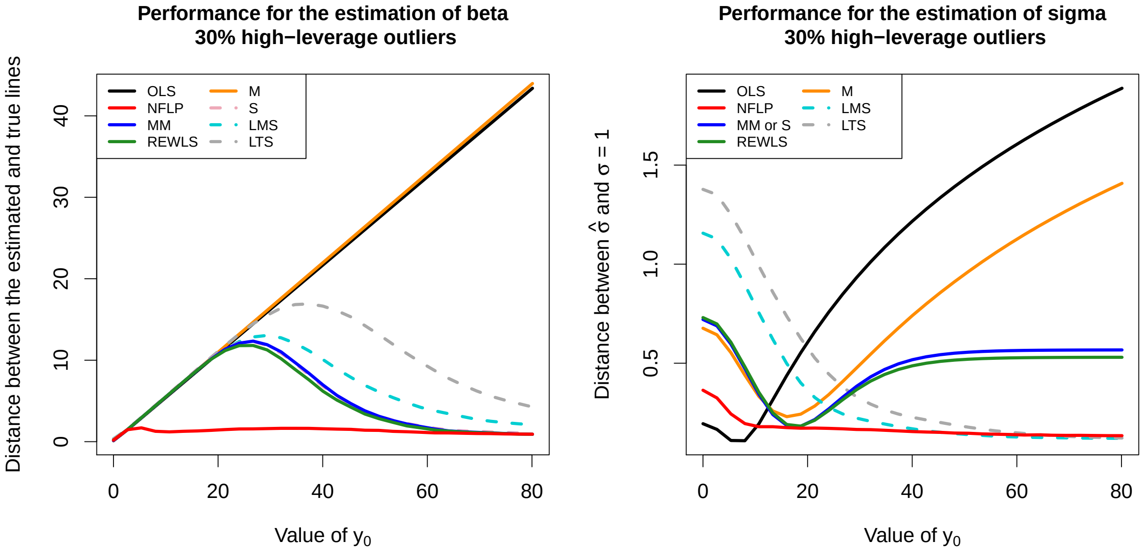


Figure 6: Performance of the estimators of $\boldsymbol{\beta}$ (left) and $\sigma$ (right) against 30% high-leverage outliers
